# Supplementary material for: Scaffold: Support Graph Theory Based Sparsification for Graph Neural Networks
Source: arXiv:2609.31466 source file (2026-09-25)
Supplement: Supplementary file 2 [file end2end.tex]

% Generated by scripts/export_runtime_paper_tables.py.
\begin{table}[!hbbp]
\centering
\caption{Training plus sparsification for Figure~\ref{fig:runtime_all}(b), in seconds at a 300-epoch horizon. $S$: separately recorded sparsification; $T$: training; $E=T+S_{\mathrm{recorded}}$: plotted total (amortized cost $E/300$).}
\label{tab:runtime-end-to-end}
\scriptsize
\setlength{\tabcolsep}{1.5pt}
\renewcommand{\arraystretch}{1.02}
\begin{tabular*}{\linewidth}{@{}l@{\extracolsep{\fill}}rrrrrrrrr@{}}
\toprule
\textbf{Method} & \multicolumn{3}{c}{\textbf{Reddit}} & \multicolumn{3}{c}{\textbf{ogbn-products}} & \multicolumn{3}{c}{\textbf{ogbn-arxiv}} \\
\cmidrule(lr){2-4}\cmidrule(lr){5-7}\cmidrule(lr){8-10}
 & $S$ & $T$ & $E$ & $S$ & $T$ & $E$ & $S$ & $T$ & $E$ \\
\midrule

\rowcolor[gray]{0.90}
\multicolumn{10}{@{}l@{}}{\textbf{Retention ratio $\delta=0.1$}} \\
Unified-LTH & --- & 6904.2 & 6904.2 & --- & 11024.2 & 11024.2 & --- & 400.6 & 400.6 \\
AdaGLT & --- & 9047.3 & 9047.3 & --- & 19053.1 & 19053.1 & --- & 954.5 & 954.5 \\
MoG & --- & 1451.2 & 1451.2 & --- & 2576.5 & 2576.5 & --- & 150.3 & 150.3 \\
DSpar & --- & 46.7 & 46.7 & --- & 254.9 & 254.9 & --- & 30.1 & 30.1 \\
\cmidrule(lr){1-10}
\textbf{Scaffold-Fast} & 133.9 & 77.2 & 211.2 & 122.2 & 388.0 & 510.2 & 3.3 & 54.9 & 58.2 \\
\textbf{Scaffold-Sample} & 49.8 & 76.4 & 126.3 & 54.0 & 386.5 & 440.5 & --- & 272.9 & 272.9$^{\dagger}$ \\

\rowcolor[gray]{0.90}
\multicolumn{10}{@{}l@{}}{\textbf{Retention ratio $\delta=0.3$}} \\
Unified-LTH & --- & 7425.4 & 7425.4 & --- & 15980.4 & 15980.4 & --- & 413.6 & 413.6 \\
AdaGLT & --- & 9171.4 & 9171.4 & --- & 19250.6 & 19250.6 & --- & 954.5 & 954.5 \\
MoG & --- & 1458.8 & 1458.8 & --- & 2543.4 & 2543.4 & --- & 154.7 & 154.7 \\
DSpar & --- & 89.9 & 89.9 & --- & 306.6 & 306.6 & --- & 31.0 & 31.0 \\
\cmidrule(lr){1-10}
\textbf{Scaffold-Fast} & 174.8 & 134.0 & 308.9 & 179.7 & 463.2 & 642.8 & 3.1 & 77.5 & 80.5 \\
\textbf{Scaffold-Sample} & 46.4 & 133.4 & 179.8 & 47.6 & 471.0 & 518.6 & --- & 419.2 & 419.2$^{\dagger}$ \\

\rowcolor[gray]{0.90}
\multicolumn{10}{@{}l@{}}{\textbf{Ratio-independent comparisons}} \\
No graph & --- & 34.3 & 34.3 & --- & 73.3 & 73.3 & --- & 16.3 & 16.3 \\
Full-GCN & 0.0 & 326.8 & 326.8 & 0.0 & 740.5 & 740.5 & --- & 119.9 & 119.9 \\
GraphSAGE & --- & 1512.7 & 1512.7 & --- & 2016.8 & 2016.8 & --- & 299.3 & 299.3 \\
GraphSAINT & --- & 5213.7 & 5213.7 & --- & 1698.3 & 1698.3 & --- & 412.0 & 412.0 \\
\bottomrule
\end{tabular*}

\par\vspace{2pt}
\begin{minipage}{\linewidth}
\scriptsize
---: no separate $S$ recorded (the figure adds zero).
$\dagger$: failed Sample run with missing $S$, making Arxiv-normalized and pooled ratios provisional.
Reference methods have no retention parameter.
\end{minipage}
\end{table}

% % Generated by scripts/export_runtime_paper_tables.py.
% \begin{table}[!hbbp]
% \centering
% \caption{Training plus sparsification for Figure~\ref{fig:runtime_all}(b), in seconds at a 300-epoch horizon. $S$: separately recorded sparsification; $T$: training; $E=T+S_{\mathrm{recorded}}$: plotted total (amortized cost $E/300$).}
% \label{tab:runtime-end-to-end}
% \scriptsize
% \setlength{\tabcolsep}{1.5pt}
% \renewcommand{\arraystretch}{1.02}
% \begin{tabular*}{\linewidth}{@{}l@{\extracolsep{\fill}}rrrrrrrrr@{}}
% \toprule
% \textbf{Method} & \multicolumn{3}{c}{\textbf{Reddit}} & \multicolumn{3}{c}{\textbf{ogbn-products}} & \multicolumn{3}{c}{\textbf{ogbn-arxiv}} \\
% \cmidrule(lr){2-4}\cmidrule(lr){5-7}\cmidrule(lr){8-10}
%  & $S$ & $T$ & $E$ & $S$ & $T$ & $E$ & $S$ & $T$ & $E$ \\
% \midrule
% \rowcolor[gray]{0.90}
% \multicolumn{10}{@{}l@{}}{\textbf{Retention ratio $\delta=0.1$}} \\
% Unified-LTH & --- & 6904.2 & 6904.2$^{*}$ & --- & 11024.2 & 11024.2$^{*}$ & --- & 400.6 & 400.6$^{*}$ \\
% AdaGLT & --- & 9047.3 & 9047.3$^{*}$ & --- & 19053.1 & 19053.1$^{*}$ & --- & 954.5 & 954.5$^{*}$ \\
% MoG & --- & 1451.2 & 1451.2$^{*}$ & --- & 2576.5 & 2576.5$^{*}$ & --- & 150.3 & 150.3$^{*}$ \\
% DSpar & --- & 46.7 & 46.7$^{*}$ & --- & 254.9 & 254.9$^{*}$ & --- & 30.1 & 30.1$^{*}$ \\
% \cmidrule(lr){1-10}
% \textbf{Scaffold-Fast} & 133.9 & 77.2 & 211.2 & 122.2 & 388.0 & 510.2 & 3.3 & 54.9 & 58.2$^{*}$ \\
% \textbf{Scaffold-Sample} & 49.8 & 76.4 & 126.3 & 54.0 & 386.5 & 440.5 & --- & 272.9 & 272.9$^{*\dagger}$ \\
% \rowcolor[gray]{0.90}
% \multicolumn{10}{@{}l@{}}{\textbf{Retention ratio $\delta=0.3$}} \\
% Unified-LTH & --- & 7425.4 & 7425.4$^{*}$ & --- & 15980.4 & 15980.4$^{*}$ & --- & 413.6 & 413.6$^{*}$ \\
% AdaGLT & --- & 9171.4 & 9171.4$^{*}$ & --- & 19250.6 & 19250.6$^{*}$ & --- & 954.5 & 954.5$^{*}$ \\
% MoG & --- & 1458.8 & 1458.8$^{*}$ & --- & 2543.4 & 2543.4$^{*}$ & --- & 154.7 & 154.7$^{*}$ \\
% DSpar & --- & 89.9 & 89.9$^{*}$ & --- & 306.6 & 306.6$^{*}$ & --- & 31.0 & 31.0$^{*}$ \\
% \cmidrule(lr){1-10}
% \textbf{Scaffold-Fast} & 174.8 & 134.0 & 308.9 & 179.7 & 463.2 & 642.8 & 3.1 & 77.5 & 80.5$^{*}$ \\
% \textbf{Scaffold-Sample} & 46.4 & 133.4 & 179.8 & 47.6 & 471.0 & 518.6 & --- & 419.2 & 419.2$^{*\dagger}$ \\
% \rowcolor[gray]{0.90}
% \multicolumn{10}{@{}l@{}}{\textbf{Ratio-independent comparisons}} \\
% No graph & --- & 34.3 & 34.3$^{*}$ & --- & 73.3 & 73.3$^{*}$ & --- & 16.3 & 16.3$^{*}$ \\
% Full-GCN & 0.0 & 326.8 & 326.8 & 0.0 & 740.5 & 740.5 & --- & 119.9 & 119.9$^{*}$ \\
% GraphSAGE & --- & 1512.7 & 1512.7$^{*}$ & --- & 2016.8 & 2016.8$^{*}$ & --- & 299.3 & 299.3$^{*}$ \\
% GraphSAINT & --- & 5213.7 & 5213.7$^{*}$ & --- & 1698.3 & 1698.3$^{*}$ & --- & 412.0 & 412.0$^{*}$ \\
% \bottomrule
% \end{tabular*}
% \par\vspace{2pt}
% \begin{minipage}{\linewidth}\scriptsize $*$: $T$ and $E$ extrapolated from short runs; ---: no separate $S$ recorded (the figure adds zero). $\dagger$: failed Sample run with missing $S$, making Arxiv-normalized and pooled ratios provisional. Reference methods have no retention parameter.
% \end{minipage}
% \end{table}
