# Supplementary material for: Scaffold: Support Graph Theory Based Sparsification for Graph Neural Networks
Source: arXiv:2609.31466 source file (2026-09-25)
Supplement: Supplementary file 3 [file workers.tex]

% Generated by scripts/export_runtime_paper_tables.py.
\begin{table}[!htbp]
\centering
\caption{Support-generation time (s) versus CPU workers at $\delta=0.3$ in Figure~\ref{fig:runtime_profiling}.}
\label{tab:runtime-workers}
\scriptsize
\setlength{\tabcolsep}{1.5pt}
\renewcommand{\arraystretch}{1.02}
\begin{tabular*}{\linewidth}{@{}l@{\extracolsep{\fill}}rrrrrr@{}}
\toprule
\textbf{Variant} & \multicolumn{6}{c}{\textbf{CPU workers}} \\
\cmidrule(lr){2-7}
 & 1 & 2 & 4 & 8 & 16 & 32 \\
\midrule
\rowcolor[gray]{0.90}
\multicolumn{7}{@{}l@{}}{\textbf{\textsc{reddit}}} \\
\textbf{Fast} & 518.3 & 300.4 & 242.6 & 216.0 & 189.5 & 178.4 \\
\textbf{Batch} & 653.9 & 381.8 & 304.1 & 285.7 & 234.3 & 229.0 \\
\textbf{Sample} & 76.7 & 27.3 & 32.0 & 25.1 & 26.2 & 26.5 \\
\rowcolor[gray]{0.90}
\multicolumn{7}{@{}l@{}}{\textbf{\textsc{ogbn-products}}} \\
\textbf{Fast} & 474.4 & 308.6 & 241.4 & 230.8 & 168.9 & 188.4 \\
\textbf{Batch} & 644.9 & 397.8 & 335.7 & 270.0 & 218.9 & 247.5 \\
\textbf{Sample} & 89.3 & 38.6 & 42.9 & 34.7 & 38.3 & 33.5 \\
\bottomrule
\end{tabular*}
\par\vspace{2pt}
\begin{minipage}{\linewidth}\scriptsize One run per setting on AMD EPYC 7502, with cached partitions/weights and warmed kernels; this sweep is separate from the training profiles.
\end{minipage}
\end{table}
